# Supplementary material for: Supply and demand shocks in the COVID-19 pandemic: An industry and occupation perspective
Source: arXiv:2004.06759 source file (2020-04-14)
Supplement: Supplementary file 1 [file table_workactivityratings_appendix.tex]

{\scriptsize
    \begin{longtable}{|l|l|}
    \hline
        Work Activity & Consensus rating \\ \hline
        Assess characteristics or impacts of regulations or policies. & 1 \\ \hline
        Advise others on legal or regulatory matters. & 1 \\ \hline
        Manage budgets or finances. & 1 \\ \hline
        Communicate with others about operational plans or activities. & 1 \\ \hline
        Analyze data to improve operations. & 1 \\ \hline
        Implement procedures or processes. & 0 \\ \hline
        Develop organizational policies, systems, or processes. & 1 \\ \hline
        Direct organizational operations, activities, or procedures. & 1 \\ \hline
        Negotiate contracts or agreements. & 1 \\ \hline
        Assign work to others. & 1 \\ \hline
        Manage human resources activities. & 1 \\ \hline
        Prepare financial documents, reports, or budgets. & 1 \\ \hline
        Prepare reports of operational or procedural activities. & 1 \\ \hline
        Resolve personnel or operational problems. & 0 \\ \hline
        Provide information or assistance to the public. & 1 \\ \hline
        Explain regulations, policies, or procedures. & 1 \\ \hline
        Coordinate activities with clients, agencies, or organizations. & 1 \\ \hline
        Direct construction or extraction activities. & 0 \\ \hline
        Coordinate group, community, or public activities. & 0 \\ \hline
        Promote products, services, or programs. & 0 \\ \hline
        Draft legislation or regulations. & 1 \\ \hline
        Identify business or organizational opportunities. & 1 \\ \hline
        Evaluate programs, practices, or processes. & 1 \\ \hline
        Prepare schedules for services or facilities. & 1 \\ \hline
        Maintain operational records. & 0 \\ \hline
        Prepare proposals or grant applications. & 1 \\ \hline
        Supervise personnel activities. & 0 \\ \hline
        Assess compliance with environmental standards or regulations. & 0 \\ \hline
        Develop business or marketing plans. & 1 \\ \hline
        Investigate the environmental impact of industrial or development activities. & 0 \\ \hline
        Evaluate project feasibility. & 1 \\ \hline
        Evaluate designs, specifications, or other technical data. & 1 \\ \hline
        Develop sustainable organizational or business policies or practices. & 1 \\ \hline
        Manage control systems or activities. & 0 \\ \hline
        Develop operational or technical procedures or standards. & 1 \\ \hline
        Analyze business or financial data. & 1 \\ \hline
        Monitor individual behavior or performance. & 0 \\ \hline
        Develop organizational or program goals or objectives. & 1 \\ \hline
        Train others on operational or work procedures. & 0 \\ \hline
        Perform recruiting or hiring activities. & 1 \\ \hline
        Provide information to guests, clients, or customers. & 0 \\ \hline
        Determine resource needs of projects or operations. & 1 \\ \hline
        Advise others on business or operational matters. & 1 \\ \hline
        Design structures or facilities. & 1 \\ \hline
        Maintain current knowledge in area of expertise. & 1 \\ \hline
        Respond to customer problems or inquiries. & 1 \\ \hline
        Develop professional relationships or networks. & 0 \\ \hline
        Provide support or encouragement to others. & 1 \\ \hline
        Authorize business activities or transactions. & 1 \\ \hline
        Evaluate personnel capabilities or performance. & 0 \\ \hline
        Develop marketing or promotional materials. & 1 \\ \hline
        Examine materials or documentation for accuracy or compliance. & 0 \\ \hline
        Collect data about consumer needs or opinions. & 1 \\ \hline
        Compile records, documentation, or other data. & 1 \\ \hline
        Advise others on products or services. & 1 \\ \hline
        Analyze market or industry conditions. & 1 \\ \hline
        Monitor external affairs, trends, or events. & 1 \\ \hline
        Evaluate the characteristics, usefulness, or performance of products or technologies. & 0 \\ \hline
        Monitor operations to ensure adequate performance. & 0 \\ \hline
        Replenish inventories of materials, equipment, or products. & 0 \\ \hline
        Purchase goods or services. & 1 \\ \hline
        Design computer or information systems or applications. & 1 \\ \hline
        Monitor financial data or activities. & 1 \\ \hline
        Monitor operations to ensure compliance with regulations or standards. & 0 \\ \hline
        Perform human resources activities. & 1 \\ \hline
        Prepare legal or regulatory documents. & 1 \\ \hline
        Examine financial activities, operations, or systems. & 1 \\ \hline
        Collect fares or payments. & 0 \\ \hline
        Analyze business or financial risks. & 1 \\ \hline
        Evaluate production inputs or outputs. & 0 \\ \hline
        Develop technical specifications for products or operations. & 0 \\ \hline
        Inspect facilities or equipment. & 0 \\ \hline
        Communicate environmental or sustainability information. & 1 \\ \hline
        Maintain tools or equipment. & 0 \\ \hline
        Prepare documentation for contracts, applications, or permits. & 1 \\ \hline
        Monitor equipment operation. & 0 \\ \hline
        Operate energy production or distribution equipment. & 0 \\ \hline
        Evaluate green technologies or processes. & 0 \\ \hline
        Schedule operational activities. & 1 \\ \hline
        Advise others on environmental sustainability or green practices. & 1 \\ \hline
        Interview people to obtain information. & 1 \\ \hline
        Develop safety standards, policies, or procedures. & 0 \\ \hline
        Investigate incidents or accidents. & 0 \\ \hline
        Develop contingency or emergency response plans. & 1 \\ \hline
        Monitor resources or inventories. & 0 \\ \hline
        Develop plans for managing or preserving natural resources. & 1 \\ \hline
        Advise others on educational or vocational matters. & 1 \\ \hline
        Manage agricultural or forestry operations. & 0 \\ \hline
        Perform agricultural activities. & 0 \\ \hline
        Estimate project development or operational costs. & 1 \\ \hline
        Develop educational programs, plans, or procedures. & 1 \\ \hline
        Teach academic or vocational subjects. & 1 \\ \hline
        Direct security or safety activities or operations. & 0 \\ \hline
        Advise others on financial matters. & 1 \\ \hline
        Execute financial transactions. & 1 \\ \hline
        Determine values or prices of goods or services. & 1 \\ \hline
        Evaluate condition of financial assets, property, or other resources. & 1 \\ \hline
        Communicate with others about business strategies. & 1 \\ \hline
        Obtain information about goods or services. & 1 \\ \hline
        Investigate criminal or legal matters. & 0 \\ \hline
        Evaluate the quality or accuracy of data. & 1 \\ \hline
        Gather information from physical or electronic sources. & 0 \\ \hline
        Verify personal information. & 0 \\ \hline
        Present information in legal proceedings. & 0 \\ \hline
        Present research or technical information. & 1 \\ \hline
        Research organizational behavior, processes, or performance. & 1 \\ \hline
        Coordinate regulatory compliance activities. & 1 \\ \hline
        Record information about legal matters. & 1 \\ \hline
        Obtain formal documentation or authorization. & 1 \\ \hline
        Prepare informational or instructional materials. & 1 \\ \hline
        Distribute materials, supplies, or resources. & 0 \\ \hline
        Develop financial or business plans. & 1 \\ \hline
        Gather data about operational or development activities. & 1 \\ \hline
        Explain financial information. & 1 \\ \hline
        Create visual designs or displays. & 1 \\ \hline
        Calculate financial data. & 1 \\ \hline
        Communicate with others about specifications or project details. & 1 \\ \hline
        Coordinate with others to resolve problems. & 1 \\ \hline
        Analyze scientific or applied data using mathematical principles. & 1 \\ \hline
        Train others to use equipment or products. & 0 \\ \hline
        Monitor operation of computer or information technologies. & 1 \\ \hline
        Maintain electronic, computer, or other technical equipment. & 0 \\ \hline
        Direct scientific or technical activities. & 0 \\ \hline
        Advise others on the design or use of technologies. & 1 \\ \hline
        Test performance of computer or information systems. & 1 \\ \hline
        Program computer systems or production equipment. & 1 \\ \hline
        Set up computer systems, networks, or other information systems. & 0 \\ \hline
        Document technical designs, procedures, or activities. & 1 \\ \hline
        Read documents or materials to inform work processes. & 1 \\ \hline
        Resolve computer problems. & 1 \\ \hline
        Analyze health or medical data. & 1 \\ \hline
        Implement security measures for computer or information systems. & 1 \\ \hline
        Research technology designs or applications. & 1 \\ \hline
        Develop research plans or methodologies. & 1 \\ \hline
        Develop models of systems, processes, or products. & 1 \\ \hline
        Process digital or online data. & 1 \\ \hline
        Design databases. & 1 \\ \hline
        Plan work activities. & 1 \\ \hline
        Analyze performance of systems or equipment. & 0 \\ \hline
        Analyze environmental or geospatial data. & 1 \\ \hline
        Develop scientific or mathematical theories or models. & 1 \\ \hline
        Determine operational methods or procedures. & 1 \\ \hline
        Confer with clients to determine needs or order specifications. & 1 \\ \hline
        Develop systems or practices to mitigate or resolve environmental problems. & 1 \\ \hline
        Select materials or equipment for operations or projects. & 1 \\ \hline
        Assess characteristics of land or property. & 0 \\ \hline
        Inspect completed work or finished products. & 0 \\ \hline
        Operate computer systems or computerized equipment. & 0 \\ \hline
        Adjust equipment to ensure adequate performance. & 0 \\ \hline
        Test performance of equipment or systems. & 0 \\ \hline
        Design electrical or electronic systems or equipment. & 1 \\ \hline
        Investigate organizational or operational problems. & 0 \\ \hline
        Inspect commercial, industrial, or production systems or equipment. & 0 \\ \hline
        Design industrial systems or equipment. & 1 \\ \hline
        Install commercial or production equipment. & 0 \\ \hline
        Diagnose system or equipment problems. & 0 \\ \hline
        Test characteristics of materials or products. & 0 \\ \hline
        Advise others on workplace health or safety issues. & 0 \\ \hline
        Assemble equipment or components. & 0 \\ \hline
        Monitor environmental conditions. & 0 \\ \hline
        Teach safety procedures or standards to others. & 0 \\ \hline
        Package objects. & 0 \\ \hline
        Assist scientists, scholars, or technical specialists with projects or research. & 1 \\ \hline
        Explain technical details of products or services. & 1 \\ \hline
        Fabricate devices or components. & 0 \\ \hline
        Design materials or devices. & 1 \\ \hline
        Operate industrial processing or production equipment. & 0 \\ \hline
        Collect samples of products or materials. & 0 \\ \hline
        Operate laboratory or field equipment. & 0 \\ \hline
        Measure physical characteristics of materials, products, or equipment. & 0 \\ \hline
        Clean tools, equipment, facilities, or work areas. & 0 \\ \hline
        Dispose of waste or debris. & 0 \\ \hline
        Prepare industrial materials for processing or use. & 0 \\ \hline
        Research agricultural processes or practices. & 0 \\ \hline
        Research biological or ecological phenomena. & 0 \\ \hline
        Research issues related to earth sciences. & 0 \\ \hline
        Analyze biological or chemical substances or related data. & 0 \\ \hline
        Collect environmental or biological samples. & 0 \\ \hline
        Care for plants or animals. & 0 \\ \hline
        Prepare specimens or materials for testing. & 0 \\ \hline
        Mediate disputes. & 0 \\ \hline
        Plan events or programs. & 1 \\ \hline
        Research historical or social issues. & 1 \\ \hline
        Collect information about patients or clients. & 0 \\ \hline
        Record images with photographic or audiovisual equipment. & 0 \\ \hline
        Advise others on healthcare or wellness issues. & 1 \\ \hline
        Set up equipment. & 0 \\ \hline
        Counsel others about personal matters. & 1 \\ \hline
        Diagnose health conditions or disorders. & 0 \\ \hline
        Clean workpieces, finished products, or other objects. & 0 \\ \hline
        Arrange displays or decorations. & 0 \\ \hline
        Administer diagnostic tests to assess patient health. & 0 \\ \hline
        Maintain health or medical records. & 0 \\ \hline
        Develop patient or client care or treatment plans. & 0 \\ \hline
        Monitor health conditions of humans or animals. & 0 \\ \hline
        Confer with healthcare or other professionals about patient care. & 1 \\ \hline
        Assist others to access additional services or resources. & 0 \\ \hline
        Advocate for individual or community needs. & 0 \\ \hline
        Explain medical information to patients or family members. & 1 \\ \hline
        Develop public or community health programs. & 1 \\ \hline
        Collaborate in the development of educational programs. & 1 \\ \hline
        Assess living, work, or social needs or status of individuals or communities. & 0 \\ \hline
        Teach life skills. & 1 \\ \hline
        Assist individuals with special needs. & 0 \\ \hline
        Research healthcare issues. & 1 \\ \hline
        Administer basic health care or medical treatments. & 0 \\ \hline
        Develop health assessment methods or programs. & 1 \\ \hline
        Transport patients or clients. & 0 \\ \hline
        Interpret language, cultural, or religious information for others. & 1 \\ \hline
        Research laws, precedents, or other legal data. & 1 \\ \hline
        Consult legal materials or public records. & 1 \\ \hline
        Discuss legal matters with clients, disputants, or legal professionals or staff. & 0 \\ \hline
        Direct legal activities. & 0 \\ \hline
        Perform court-related or other legal administrative activities. & 0 \\ \hline
        Make legal decisions. & 1 \\ \hline
        Assess student capabilities, needs, or performance. & 1 \\ \hline
        Perform administrative or clerical activities. & 1 \\ \hline
        Serve on organizational committees. & 1 \\ \hline
        Write material for artistic or commercial purposes. & 1 \\ \hline
        Evaluate scholarly work. & 1 \\ \hline
        Edit written materials or documents. & 1 \\ \hline
        Set up classrooms, facilities, educational materials, or equipment. & 0 \\ \hline
        Train others on health or medical topics. & 0 \\ \hline
        Inspect characteristics or conditions of materials or products. & 0 \\ \hline
        Provide general assistance to others, such as customers, patrons, or motorists. & 0 \\ \hline
        Build structures. & 0 \\ \hline
        Operate audiovisual or related equipment. & 0 \\ \hline
        Study details of artistic productions. & 1 \\ \hline
        Coordinate artistic or entertainment activities. & 0 \\ \hline
        Create artistic designs or performances. & 0 \\ \hline
        Create decorative objects or parts of objects. & 0 \\ \hline
        Apply decorative finishes. & 0 \\ \hline
        Assemble products or work aids. & 0 \\ \hline
        Present arts or entertainment performances. & 0 \\ \hline
        Perform athletic activities for fitness, competition, or artistic purposes. & 0 \\ \hline
        Develop news, entertainment, or artistic content. & 1 \\ \hline
        Alter audio or video recordings. & 1 \\ \hline
        Operate communications equipment or systems. & 0 \\ \hline
        Coach others. & 0 \\ \hline
        Gather information for news stories. & 1 \\ \hline
        Notify others of emergencies or problems. & 0 \\ \hline
        Mark materials or objects for identification. & 0 \\ \hline
        Schedule appointments. & 1 \\ \hline
        Administer therapeutic treatments. & 0 \\ \hline
        Examine people or animals to assess health conditions or physical characteristics. & 0 \\ \hline
        Advise patients or clients on medical issues. & 0 \\ \hline
        Follow standard healthcare safety procedures to protect patient and staff members. & 0 \\ \hline
        Operate medical equipment. & 0 \\ \hline
        Fabricate medical devices. & 0 \\ \hline
        Adjust medical equipment to ensure adequate performance. & 0 \\ \hline
        Treat injuries, illnesses, or diseases. & 0 \\ \hline
        Prescribe medical treatments or devices. & 0 \\ \hline
        Administer emergency medical treatment. & 0 \\ \hline
        Fit assistive devices to patients or clients. & 0 \\ \hline
        Prepare mixtures or solutions. & 0 \\ \hline
        Sell products or services. & 0 \\ \hline
        Assist healthcare practitioners during medical procedures. & 0 \\ \hline
        Order medical tests or procedures. & 1 \\ \hline
        Prepare health or medical documents. & 1 \\ \hline
        Clean medical equipment or facilities. & 0 \\ \hline
        Evaluate patient or client condition or treatment options. & 0 \\ \hline
        Prepare medical equipment or work areas for use. & 0 \\ \hline
        Maintain medical equipment or instruments. & 0 \\ \hline
        Test sites or materials for environmental hazards. & 0 \\ \hline
        Escort others. & 0 \\ \hline
        Stock supplies or products. & 0 \\ \hline
        Move materials, equipment, or supplies. & 0 \\ \hline
        Supervise activities in correctional facilities. & 0 \\ \hline
        Maintain safety or security. & 0 \\ \hline
        Intervene in crisis situations or emergencies. & 0 \\ \hline
        Monitor safety or security of work areas, facilities, or properties. & 0 \\ \hline
        Operate transportation equipment or vehicles. & 0 \\ \hline
        Process forensic or legal evidence. & 0 \\ \hline
        Issue documentation. & 0 \\ \hline
        Protect people or property from threats such as fires or flooding. & 0 \\ \hline
        Record information about environmental conditions. & 0 \\ \hline
        Investigate individuals' background, behavior, or activities. & 0 \\ \hline
        Direct vehicle traffic. & 0 \\ \hline
        Develop recipes or menus. & 1 \\ \hline
        Prepare foods or beverages. & 0 \\ \hline
        Reconcile financial data. & 1 \\ \hline
        Provide food or beverage services. & 0 \\ \hline
        Cut trees or other vegetation. & 0 \\ \hline
        Operate agricultural or forestry equipment. & 0 \\ \hline
        Apply protective solutions or coatings. & 0 \\ \hline
        Maintain sales or financial records. & 1 \\ \hline
        Conduct amusement or gaming activities. & 0 \\ \hline
        Maintain facilities or equipment. & 0 \\ \hline
        Train animals. & 0 \\ \hline
        Apply hygienic or cosmetic agents to skin or hair. & 0 \\ \hline
        Embalm corpses. & 0 \\ \hline
        Groom or style hair. & 0 \\ \hline
        Sort materials or products. & 0 \\ \hline
        Assist individuals with paperwork. & 1 \\ \hline
        Operate office equipment. & 0 \\ \hline
        Process shipments or mail. & 0 \\ \hline
        Load products, materials, or equipment for transportation or further processing. & 0 \\ \hline
        Process animal carcasses. & 0 \\ \hline
        Hunt animals. & 0 \\ \hline
        Position tools or equipment. & 0 \\ \hline
        Position materials or components for assembly. & 0 \\ \hline
        Perform general construction or extraction activities. & 0 \\ \hline
        Join parts using soldering, welding, or brazing techniques. & 0 \\ \hline
        Operate lifting or moving equipment. & 0 \\ \hline
        Signal others to coordinate work activities. & 0 \\ \hline
        Cut materials. & 0 \\ \hline
        Apply materials to fill gaps or imperfections. & 0 \\ \hline
        Smooth surfaces of objects or equipment. & 0 \\ \hline
        Drill holes in earth or materials. & 0 \\ \hline
        Operate construction or excavation equipment. & 0 \\ \hline
        Disassemble equipment. & 0 \\ \hline
        Install plumbing or piping equipment or systems. & 0 \\ \hline
        Operate pumping systems or equipment. & 0 \\ \hline
        Set up protective structures or coverings near work areas. & 0 \\ \hline
        Climb equipment or structures. & 0 \\ \hline
        Repair electrical or electronic equipment. & 0 \\ \hline
        Connect components or supply lines to equipment or tools. & 0 \\ \hline
        Install energy or heating equipment. & 0 \\ \hline
        Repair tools or equipment. & 0 \\ \hline
        Maintain vehicles in working condition. & 0 \\ \hline
        Repair vehicle components. & 0 \\ \hline
        Inspect vehicles. & 0 \\ \hline
        Sew garments or materials. & 0 \\ \hline
        Operate cutting or grinding equipment. & 0 \\ \hline
        Repair workpieces or products. & 0 \\ \hline
        Shape materials to create products. & 0 \\ \hline
        Position workpieces or materials on equipment. & 0 \\ \hline
        Remove workpieces from production equipment. & 0 \\ \hline
        Engrave objects. & 0 \\ \hline
        Take physical measurements of patients or clients. & 0 \\ \hline
        Monitor traffic conditions. & 0 \\ \hline
        Tend watercraft. & 0 \\ \hline
            \caption{{\bf Work activities and their consensus rating as to whether they can be performed at home.} }
    \label{tab:work_activity_ratings}        
    \end{longtable}
}
